# Supplementary material for: Path Planning with Uncertainty for Aircraft Under Threat of Detection from Ground-Based Radar
Source: arXiv:2207.03716 source file (2022-07-08)
Supplement: Supplementary file 1 [file Appendices.tex]

%
%  Section: RCS Azimuth and Elevation Angle
%
This appendix section provides the derivation for the RCS azimuth $\alpha$ and elevation $\phi$ angles used in the ellipsoid RCS model in \eqref{eq:rcs_ellipsoid}.
The RCS model used on this paper provides an expression for the RCS value as a function of the azimuth and elevation angles of the radar detection vector in the body frame of the aircraft.
The body frame $x$ and $y$ axes are shown as $b_x$ and $b_y$ in Fig. \ref{fig:radar_xy} and the body frame $z$ axis points out of the bottom of the aircraft.
Let the aircraft position in the NED frame and the aircraft attitude be defined as
\begin{eqnarray}
    \boldsymbol{p_a^n} &=& \begin{bmatrix} p_{an} & p_{ae} & p_{ad} \end{bmatrix}^\intercal \label{eq:pa} \\
    \boldsymbol{\Theta_a} &=& \begin{bmatrix} \phi_a & \theta_a & \psi_a \end{bmatrix}^\intercal \label{eq:theta_a}
\end{eqnarray}
and the radar position in the NED frame be defined as
\begin{equation}
    \boldsymbol{p_r^n} = \begin{bmatrix} p_{rn} & p_{re} & p_{rd}\end{bmatrix}^\intercal. 
\end{equation}
The position of the radar in the body frame of the aircraft is given by
\begin{equation}
\boldsymbol{\rho_r^b} = \begin{bmatrix} \rho_{rx} & \rho_{ry} & \rho_{rz} \end{bmatrix}^\intercal.
\end{equation}
The vector $\boldsymbol{\rho_r^b}$ is calculated using the aircraft pose and radar position by
\begin{equation}
    \boldsymbol{\rho_r^b} = T_n^b \left(\boldsymbol{p_r^n}-\boldsymbol{p_a^n}\right)
\end{equation}
where $T_n^b$ is the direction cosine matrix formed by the ZYX Euler angle sequence \cite{beard_randy_small_2012} given by
\begin{align}
    T_n^b = &\left[\begin{matrix}  C{\psi_a} C{\theta_a} & -C{\phi_a} S{\psi_a} + C{\psi_a} S{\phi_a} S{\theta_a}  \\
                C{\theta_a} S{\psi_a} & C{\phi_a} C{\psi_a} + S{\phi_a} S{\psi_a} S{\theta_a}  \\
                -S{\theta_a} & C{\theta_a} S{\phi_a} \end{matrix}\right.\nonumber \\
        & \qquad \qquad \qquad \qquad \left.\begin{matrix}
        S{\phi_a} S{\psi_a} + C{\phi_a}C{\psi_a}S{\theta_a} \\
        -C{\psi_a} S{\phi_a} + C{\phi_a} S{\psi_a} S{\theta_a} \\
        C{\phi_a} C{\theta_a} \end{matrix}\right] \label{eq:DCM_zyx}
\end{align}
and $\textrm{S}\cdot$ and $\textrm{C}\cdot$ are the $\sin(\cdot)$ and $\cos(\cdot)$ functions.

The RCS azimuth angle is the angle from the body frame $x$ axis to the projection of the radar detection vector into the $x$-$y$ plane of the body frame given by 
\begin{eqnarray}
    \alpha &=& \arctan\left(\frac{\rho_{ry}}{\rho_{rx}}\right).
\end{eqnarray}
The RCS elevation angle $\phi$ is the angle from the $x$-$y$ plane in the body frame of the aircraft to the radar detection vector with a positive angle towards the bottom of the aircraft given by
\begin{eqnarray}
    \phi &=& \arctan\left(\frac{\rho_{rz}}{\sqrt{(\rho_{rx})^2+(\rho_{ry})^2}}\right).
\end{eqnarray}
